# Supplementary material for: Offline Policy Optimization in RL with Variance Regularizaton
Source: arXiv:2212.14405 source file (2022-12-29)
Supplement: Supplementary file 1 [file appendix_bilevel_opt.tex]

\section{Estimating Distribution Ratio in Offline Policy Optimization - Bi-Level Optimization Perspective}

To optimize the off-policy optimization problem with state-action distribution corrections effectively, we can view this as an alternating dual optimization problem such that the resulting algorithm can converge to a unique Nash equilibrium, ie, $(\pi, \mu) = (\pi^{*}, \pi^{*})$. For the bi-level optimization perspective and analysis in this section, we assume we have access to the data logging policy $\mu$ which collects the batch data $\mathcal{D}$.
The off-policy optimization objective often takes the form : 
\begin{align}
\label{eq:trpo_objective_offpolicy}
    J(\pi_\theta) = \mathbb{E}_{(s,a) \sim d_{\mathcal{D}}(s,a)}\biggl[ \frac{d_{\pi_{\theta}}(s, a)}{d_{\mathcal{D}} (s, a)}\cdot Q(s,a) \biggr]
    - \beta \cdot  \mathcal{D}_{f}(d_{\pi} || d_{\mathcal{D}}) 
\end{align}
where for clarity of understand, we have additionally introduced the divergence regularizer term $\mathcal{D}_{f}(d_{\pi} || d_{\mathcal{D}})$. Note that similar regularizers of this form has also been considered in offline algorithms such as AlgaeDICE \citep{AlgaeDICE}. 

In the outer loop optimization, we update $\pi$ using samples under $d_{\mathcal{D}}(s,a)$ where we perform policy optimization regularizing with the behaviour policy. In the following sections, we show that we can formulate an overall dual off-policy optimization problem, where in the primal form, we solve for the policy gradient objective with off-policy data under $\mu$, and in the dual form solve for the dual variables to estimate the distribution ratio required for the local distribution matching step.

\textit{Inner Optimization : Distribution Matching : } Under our alternating minimax formulation, we first perform a \textit{local} imitation learning or distribution matching step that involves estimating or correcting for the ratio between state-action distributions $d_{\pi}$ and $d_{\mu}$. We introduce a dual transformation using Fenchel duality, inspired from \citep{DualDICE, SBEED, 2019GENDICEGO}, such that optimizing the dual function is equivalent to estimating the distribution ratio. This leads to an optimization objective
\begin{equation}
    \max_{h} \quad \mathcal{J}_{\text{GAIL}}(h) = \mathbb{E}_{(s,a) \sim d_{\pi}} \Big[ \log h(s,a)  \Big] +
    \mathbb{E}_{(s,a) \sim d_{\mu}} \Big[ \log (1 - h(s,a))   \Big], 
\end{equation}
similar to GAIL \citep{GAIL}, where $h$ is the discriminator function to discriminate between the samples of $d_{\pi}$ and $d_{\mu}$. The local distribution matching step involves solving the dual problem which is equivalent to learning a behaviour policy $\mu$ such that it remains close to the target policy, minimizing the variance between the state-action samples under the two policies \citep{behaviour_policy_search}. The inner loop involves minimizing the KL divergence term, where we need to estimate the ratio of the state-action distributions. Considering the dual form of the KL divergence term where we introduce the dual function $\nu$, such that the $- \text{KL} = \min_{x} \mathcal{K}_{\text{DICE}}$, given by :
\begin{align*}
\label{eq:kl_duality}
       & - \text{KL}( d_{\mathcal{D}}(s,a) || d_{\pi}(s,a) ) = 
       & \underset{x}{\text{min}} \quad \mathbb{E}_{s \sim d_{\pi}(s), a \sim \pi(a,s)} \Big[ \exp{  x(s,a)  }    \Big] 
       & - \mathbb{E}_{s,a \sim d_{\mathcal{D}(s,a)}} \Big[  x(s,a) \Big] 
\end{align*}

\textit{Change of Variables : } The first term is based on an expectation w.r.t $d_{\pi}(s)$ which we do not have access to in practice. Using the change of variables trick, as in \citep{DualDICE}, we can transform this distribution to be  over the initial state distribution. Let us use an arbitrary variable $\nu(s,a) : \mathcal{S} \times \mathcal{A} \leftarrow \mathcal{R}$, which is an arbitrary state-action distribution that satisfies $\nu(s,a) = x(s,a) + \gamma \mathbb{E}_{s' \mid s, a} \Big[  \nu(s',a') \Big]$. We therefore have : 
\[
    \mathbb{E}_{(s, a) \sim d_{\pi}(s,a)} \Big[ x(s,a) \Big] = (1 - \gamma) \mathbb{E}_{s \sim \beta, a \sim \pi(s)} \Big[ \nu(s,a)  \Big]
\]
We therefore introduce the dual function $\nu(s,a)$ which has a similar form as the value function with the Bellman-like operator $\mathcal{B}^{\pi} = \gamma \mathbb{E}_{s' \sim P, a' \sim \pi(\cdot \mid s'))} [ \nu(s', a') ]$. By applying the change of variables trick in the dual form of the $\text{KL}$ divergence, and considering the Donsker-Varadhan representation of the KL divergence term to avoid instability due to the exponential term, we therefore have : 
\begin{multline}
    - \text{KL}(d_{\mathcal{D}}(s,a) || d_{\pi}(s,a) ) = \min_{\nu} \log  \mathbb{E}_{s \sim d_{\pi}, a \sim \pi} \Big[  \exp{( \nu(s,a)  - \mathcal{B}^{\pi}(s', a')  )} \Big] \\
    -  \mathbb{E}_{s,a  \sim d_{\mathcal{D}(s,a)}} \Big[  \nu(s,a) - \mathcal{B}^{\pi}\nu(s', a')  \Big] 
\end{multline}
For the second term, we can either telescope to reduce the expectation over initial states, or compute the second term as it is, since we have access to all the past off-policy samples in the experience replay buffer. Denoting the dual form of the $\text{KL}$ divergence as $\mathcal{K}_{\text{DICE}}$, where by solving for the dual form to find optimal $\nu(s,a)$, we can compute the ratio of $d_{\pi}(s,a)$ and $d_{\mu}(s,a)$ exactly, as given by
\begin{equation}
\label{eq:optimal_dual}
    x^{*}(s,a) = \nu^{*}(s,a) - \mathcal{B}^{\pi}\nu^{*}(s', a') = \log \frac{d_{\mu}(s,a)}{d_{\pi}(s,a)}
\end{equation}
The solution from equation \ref{eq:optimal_dual} is equivalent to minimizing the $\text{KL}$ divergence. However, note that equation \ref{eq:optimal_dual} and the dual solution still depends on both $d_{\pi}$ and $d_{\mu}$, where in the off-policy case, we usually do not have access to $d_{\pi}$. Compared to this, \citep{AlgaeDICE, DualDICE} uses the off-policy batch setting where the state-action distribution can be replaced with samples from a fixed batch data. In the online off-policy case, however, this is not the case, and therefore requires an approximation. Here, we make an approximation based on the following observation that instead of taking $d_{\pi}(s,a)$ exactly, we can instead consider only the last trajectory ie, $d_{\pi_{\text{old}}(s,a)}$. In other words, we compute the optimal ratio between $d_{\mu}(s,a)$ (ie, state-action samples in the entire replay buffer) and $d_{\pi_{\text{old}}}$ where we only take the last old trajectory, to get $\log \frac{d_{\mu}(s,a)}{d_{\pi_{\text{old}}}(s,a)}$. 

\textit{Outer Optimization : Off-Policy Policy Gradient : } Following from our off-policy optimization objective in equation \ref{eq:trpo_objective_offpolicy} and applying the dual form of the KL divergence term, we get the  outer loop objective $J(\pi_{\theta}, \nu)$ under off-policy samples : 
\begin{align}
\label{eq:off_objective}
\mathcal{J}(\pi_{\theta}, \nu) = \mathbb{E}_{d_{\mathcal{D}}(s,a)} \Bigg[ \frac{d_{\pi}(s,a)}{d_{\mathcal{D}}(s,a)} \cdot r(s,a) \Bigg] 
- \lambda \mathbb{E}_{d_{\mathcal{D}(s,a)} \Bigg[ \Big[  \nu(s,a) - \gamma \mathbb{E}_{s' \mid s, a} \Big[ \nu(s', a') \Big]  \Big]   \Bigg] + \notag \\
\lambda \Bigg[   \mathbb{E}_{d_{\beta}(s,a)} \Big[ \exp{ ( \nu(s_0,a_0) )  }  \Bigg]
\end{align}
where $d_{\beta}(s,a)$ is the starting state distribution. Since from the inner loop, we can estimate the last two terms by optimizing the dual parameters $\nu(s,a)$ by minimizing the error $(\nu(s,a) - \mathcal{B}^{\pi} \nu(s,a))$, we have further shown that the optimal solution $\nu^{*}(s,a)$ gives the optimal state-action distribution ratio in the primal form, as in equation \ref{eq:optimal_dual}, from which we can further find the optimal ratio $\frac{d_{\pi}(s,a)}{d_{\mathcal{D}(s,a)}$ as it appears in the off-policy objective \ref{eq:off_objective} :
\[
\frac{d_{\pi}(s,a)}{d_{\mathcal{D}(s,a)} = \frac{1}{\exp{( x^{*}(s,a) )}} 
\]
which can be thought of as approximating the importance sampling correction term as in off-policy actor-critic \citep{OffPAC}. The solution to the dual-problem is equivalent to minimizing the discrepancy in the importance sampling correction term. Furthermore, using the optimal primal solution $x^{*}(s,a)$ or the optimal dual solution $\nu^{*}(s,a)$, we can establish that we get a lower bound to the $\text{KL}$ divergence term, in terms of the variance of the importance sampling estimation, similar to POIS \citep{POIS}

\textit{Overall Min-Max Objective:} We can write our overall objective as a min-max alternating update scheme : 
\begin{align*}
    & \min_{\nu} \max_{\theta} \mathcal{J}(\theta, \nu) = 
    \mathbb{E}_{d_{\mathcal{D}}(s,a)} \Bigg[\frac{1}{ \exp{ (\nu(s,a) - \mathcal{B}^{\pi}\nu(s, a) ) }}  \cdot r(s,a) \Bigg] \notag \\
    & - \lambda \mathbb{E}_{d_{\mathcal{D}}(s,a)} \Bigg[ \Big[  \nu(s,a) - \gamma \mathbb{E}_{s' \mid s, a} \Big[ \nu(s', a') \Big]  \Big]   \Bigg]  
    + \lambda \Bigg[   \mathbb{E}_{d_{\beta}(s,a)} \Big[ \exp{ ( \nu(s_0,a_0) )  }  \Bigg],
\end{align*}
where note that the minimization step in the above minmax formulation implicitly depends on the inner loop optimization itself, where in the inner loop we perform distribution matching between the behaviour policy $d_{\mu}(s,a)$ and the target policy $d_{\pi}(s,a)$ state-action distributions 
\begin{align*}
    - \text{KL}(d_{\mathcal{D}} || d_{\pi}) = 
    \underset{\nu : \mathcal{S \times \mathcal{A} \rightarrow \mathcal{R}}}{\text{min}} \Big \{\log  \mathbb{E}_{d_{\beta}(s,a)} \Big[   \exp{ ( \nu(s_0, a_0) )  }  \Big] 
    - \mathbb{E}_{d_{\mathcal{D}}(s,a)} \Big[ \Big(\nu(s,a) - \mathcal{B}^{\pi} \nu(s,a)  \Big)^{2}  \Big] \} 
\end{align*}
where we can find the optimal state-action distribution correction by minimizing the overall mean squared error :  
\[
    \Big( (\nu^{*} - \mathcal{B}^{\pi}\nu )(s,a) \Big) = \frac{d_{\mu}(s,a)}{d_{\pi}(s,a)}
\]

The minimax optimization problem with alternating updates can be cast as a bilevel optimization problem. Under this scheme, the solution from the inner loop matching the distributions, or equivalently finding optimal dual function, further determines the solution in the outer loop which performs a state-action distribution correction in the off-policy policy gradient. Recall that an actor-critic algorithm \citep{Konda} can also be seen as a bilevel optimization problem (see Appendix for more details). We can write our overall bilevel formulation as : 
\begin{equation}
\label{eq:bilevel_objective}
    \begin{align}
        & \underset{\pi_{\theta}}{\text{maximize}}
        & &  \mathcal{J}(\theta, \nu) =  \mathbb{E}_{d_{\mu}(s,a)} \Bigg[ \frac{1}{\nu^{*}} \cdot  Q^{\pi_{\theta}}(s,a) -  \mathcal{K}_{\text{KL}}(\nu^{*}) \Bigg]\\
        & \text{subject to}
        & & \nu^{*} = \underset{\nu}{\text{argmin}} \quad  \Big( (  \nu(s,a) - \mathcal{B}^{\pi}\nu(s,a)    )(s,a) \Big)^{2}
    \end{align}
\end{equation}
The overall off-policy policy gradient objective depends on the solution $\nu^{*}$ from the inner loop of the optimization probem, where we minimize the expected Bellman error for the dual function $\nu(s,a)$. The solution from the dual form in the inner optimization is further used in the upper level optimization for optimal corrections for the stationary distributions.

Considering non-linear function approximation, where the behaviour regularized off-policy actor-critic algorithm consists of three set of parameters, $\theta$ for the target policy, $\omega$ for the mixture of weights for $\mu_{\omega}$ and a critic approximation $Q_{\phi} \approx Q^{\pi}$. In the inner loop, in addition to optimizing for $\omega$, as in the bi-level actor-critic formulation discussed above, we would also need to minimize the Bellman error to optimize the weights for the critic estimator $\phi$. We therefore have the overall minimax optimization problem : $\min_{\nu, \phi} \max_{\theta} \mathcal{L}(\theta, \phi, \nu)$, which can be considered as a three-time scale algorithm too. However, for ease of analysis, we resort to a two time-scale update. We have the following two minimization problems, for $\phi$ and $\omega$, where first we minimize the expected Bellman error (MSBE) : 
\[
\phi^{*} = \min_{\phi}  \mathcal{G}(\phi, \theta) = \min_{\phi} || Q_{\phi} - \mathcal{T}^{\pi_{\theta}} Q_{\phi} ||_{d_{\pi}}^{2}
\]
and then alternately minimize the mean squared Bellman error, such that we can find the optimal ratio between the state-action distribution samples $\phi$, given by 
\[
\nu^{*} = \min_{\nu} \Big( (\nu - \mathcal{B}^{\pi} \nu )(s,a) \Big)^{2} 
\]
Our overall optimization problem can further be written as a bi-level optimization problem, involving a three time-scale algorithm consisting of two inner loops solving minimization problems, and an outer loop for the policy maximization step. The proposition below shows this : 

\begin{prop} An alternating optimization framework based on the objective $\mathcal{L}(\theta, \phi, \nu)$. We use $\pi_{\theta}$ as the fast policy and $\mu_{\omega}$ as the slower reactive policy. This has the equivalent bi-level optimization problem as follows

\begin{equation}
\label{eq:ac_bilevel_minmin_max}
    \begin{align}
        & \underset{\theta}{\text{maximize}}
        & & \mathcal{F}(\theta, \omega) = \mathbb{E}_{s_0, a_0 \sim \beta} \Bigg[ Q_{\omega}^{\pi_{\theta}}(s_0,a_0)   \Bigg] \\
        & \text{subject to}
        & & \phi^{*} = \min_{\phi}  \mathcal{G}(\phi, \theta) = \min_{\phi} || Q_{\phi} - \mathcal{T}^{\pi_{\theta}} Q_{\phi} ||_{d_{\pi}}^{2}, \\
        & \text{subject to}
        & & \nu^{*} = \min_{\nu} \Big( (\nu - \mathcal{B}^{\pi} \nu )(s,a) \Big)^{2} 
    \end{align}
\end{equation}

\end{prop}

\textbf{Updating $\pi_{\theta}$ :} In the maximization step for updating $\pi_{\theta}$, we can use the samples from $\mu_{\omega}$ and perform a trust region optimization approach for optimizing the off-policy gradient objective, which follows from the regular TRPO objective as usual, with the only difference being that the samples are collected under behaviour policy $\mu(a \mid s)$. 

\textbf{Distribution Matching Step:} The minimization step involves  matching between $d_{\mu}$ and $d_{\pi}$  by minimizing $\text{KL}(d_\mu) || d_{\pi_{\theta}})$, or equivalently optimizing the dual function $\nu(s,a)$, to estimate the optimal state-action distribution correction. 

\textbf{Combining Updates for $\pi_{\theta}$ and $\nu(s,a)$: } We can alternate the updates for $\nu$ (ie, minimizing Bellman-like error) and $\pi_{\theta}$ (ie, off-policy gradient update) to form a min-max optimization objective where both the policies are tightened together to guide each other's improvements similar to Dual Policy Iteration \citep{DPI}.
